# Supplementary material for: Random Telegraph Signal in a Metallic Double-Dot System
Source: arXiv:1401.1731 source file (2014-05-14)
Supplement: Supplementary file 1 [file Supplementary_4.pdf]

# Supporting Information

## Random Telegraph Signal in a Metallic Double-Dot System

*Yuval Vardi*, Avraham Guttman and Israel Bar-Joseph*

*Department of Condensed Matter Physics, Weizmann Institute of Science, Rehovot 76100, Israel*

**E-mail: yuval.vardi@weizmann.ac.il*

## Contents

S1 Methods ..... 2
S1.1 Gold nanoparticles synthesis ..... 2
S1.2 Dimer synthesis ..... 2
S1.3 Device fabrication and electrostatic trapping ..... 4
S2 Double dot simulation ..... 6
S2.1 Fit parameters ..... 8
S2.2 Charging states ..... 8
S3 Trap dynamics ..... 10
S3.1 Time auto-correlation function $g_2$ ..... 10
S4 Measurements in the Coulomb Blockade ..... 11
S5 Demonstration of Control ..... 12
S6 Numerical Calculations of the Trap Gating ..... 13
S7 References ..... 14

# S1 Methods

## S1.1 Gold nanoparticles synthesis

Gold nanoparticles (NPs) with diameter of 12 nm were prepared using the Slot and Geuze method[1] with some modifications. A solution of 80 μL 1% tannic acid and 4 ml 1% $Na_3$citrate in 16 mL double distilled water (DDW) was heated to 60 $^{\circ}$C and then added while stirring to a 60 $^{\circ}$C solution of 1 ml 1% $NaAuCl_4$ in 79 ml DDW. The mixed solution was then heated to boil for 10 min and then cooled to room temperature.

These 12 nm NPs were used as seeds for the growth of 34 nm spherical NPs: 1 ml 1% $NaAuCl_4$ was added to 95 ml DDW. The solution was heated to boil followed by simultaneously adding 0.4 ml 1% $Na_3$citrate and 3.5 ml of 12 nm NPs' solution. The mixed solution was heated to boil for 15 min and then cooled to room temperature.

The NPs were then capped by mercaptosuccinic-acid (MSA) ligands by adding 100 μl $10^{-2}$ M MSA in MeOH to 20 ml of the NPs' solution, and waiting at room temperature for 3 hours. Transmission Electron Microscopy (TEM) images of such NPs are shown in Fig. S1:

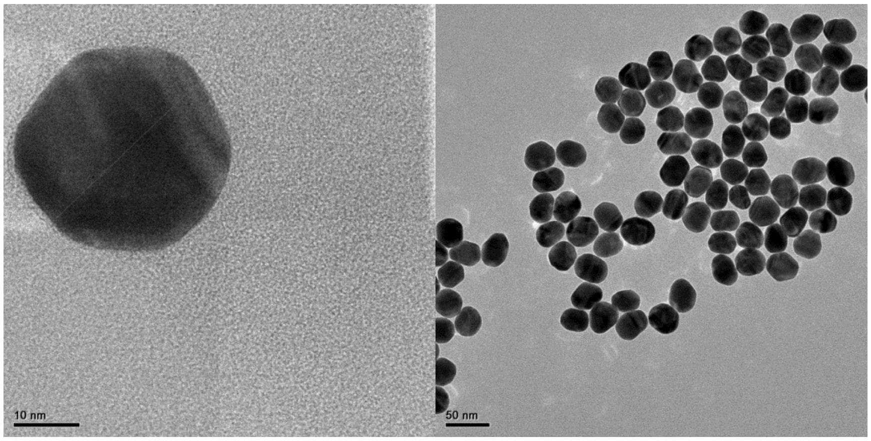


*Figure S1: TEM images of the nanoparticles*

## S1.2 Dimer synthesis

Dimers of two gold NPs, which are covalently bonded by one or more linker molecules, 4,4'-biphenyldithiol (BPD) were prepared[2,3]. 2 mg BPD was dissolved in 910 μl acetonitrile and then diluted by DDW to a final concentration of $5\cdot 10^{-7}$ M. The MSA capped 34 nm NPs was concentrated to $5\cdot 10^{-8}$ M by centrifuging the solution at 250 g for 35 min @ 4 $^{\circ}$C, and discarding the supernatant. Following, 5 μl of the diluted BPD, 1 μl $10^{-4}$ M tris(2 carboxyethyl)phosphine (TCEP) and 1 μl 10 mM NaCl were added to 5 μl of the MSA capped NPs, waiting 8 hours at room temperature in dark. In order to extract the dimers, the solution was loaded on an agarose gel that was prepared using 0.5X Tris/Borate/EDTA (TBE). The bottom band in Fig. S2 corresponds to single NPs and the top band to dimers:

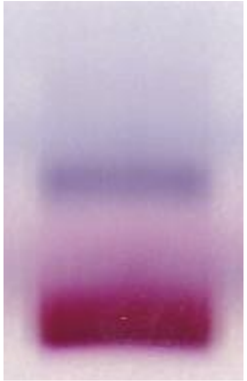

*Figure S2: Gel electrophoresis of the dimer solution.*

The extraction of the dimers out of the corresponding band in the gel is again done by another electrophoresis process, this time with a lower salinity buffer, 0.05X TBE. The lower salinity buffer is needed for the electrostatic trapping stage (S1.3).

TEM images of the extracted dimers are shown in Fig. S3:

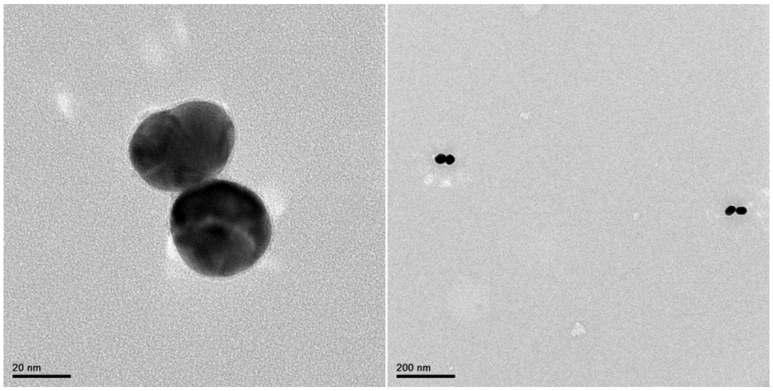


*Figure S3: TEM images showing the dimers*

Dimers can also be formed at lower yield and control without using a linking molecule. This is done using the same procedure with a higher NaCl concentration. The polar solution screens the repulsive interaction between the nanoparticles and allows them to form high order complexes. Using gel electrophoresis we can extract the spontaneously formed dimers from this solution.

## S1.3 Device fabrication and electrostatic trapping

Gold electrodes with a thickness of 25 nm and gap of 25 nm were fabricated on a heavily doped Si substrate, covered by 100 nm insulating $SiO_2$, using electron-beam (e-beam) lithography. A layer of 2 nm Nickel was used as an adhesion layer for the electrodes.

Dimers were connected to the electrodes using an electrostatic trapping method[4]. An alternating voltage of 1 V at 10 MHz was applied for 60 sec between the two electrodes, after covering them with a droplet of the dimers' solution. The dimers are then trapped in the gap between the electrodes, where the electric field magnitude is larger.

Scanning Electron Microscopy (SEM) images of trapped dimers of different devices are shown in Fig. S4:

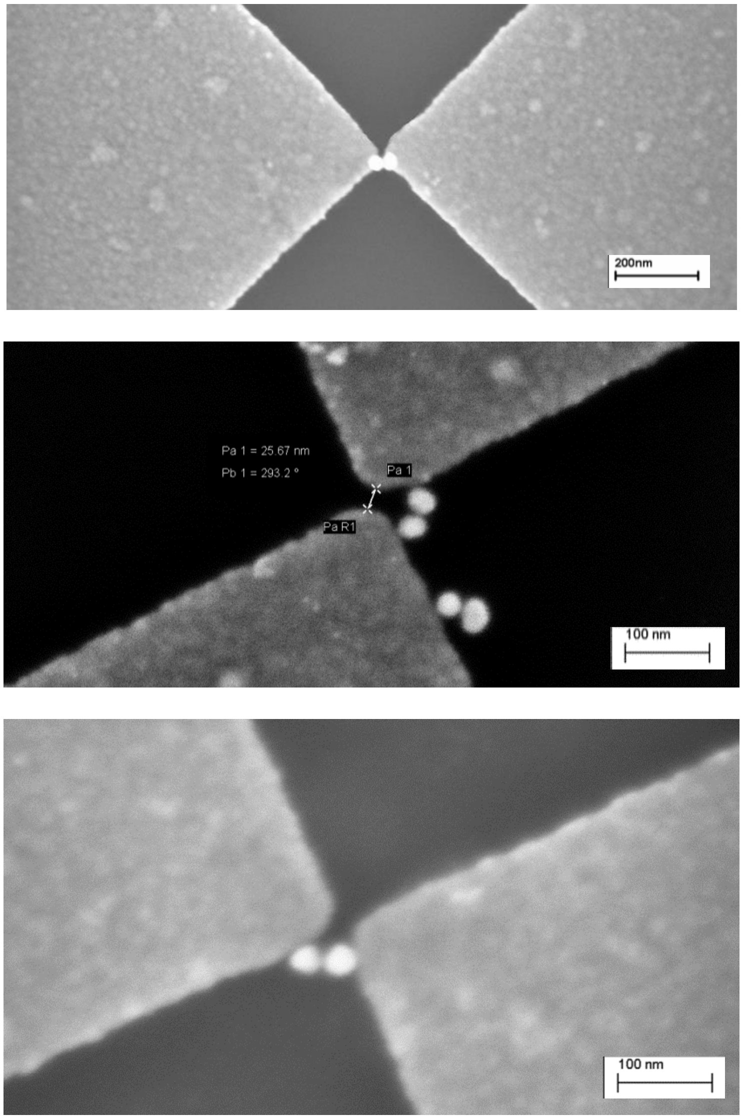


*Figure S4: Trapped dimers in different devices*

Atomic Force Microscopy (AFM) is then used to image the devices non-destructively and select the ones, which appropriately bridge the electrodes (typically, one of three dimers), see Fig. S5.

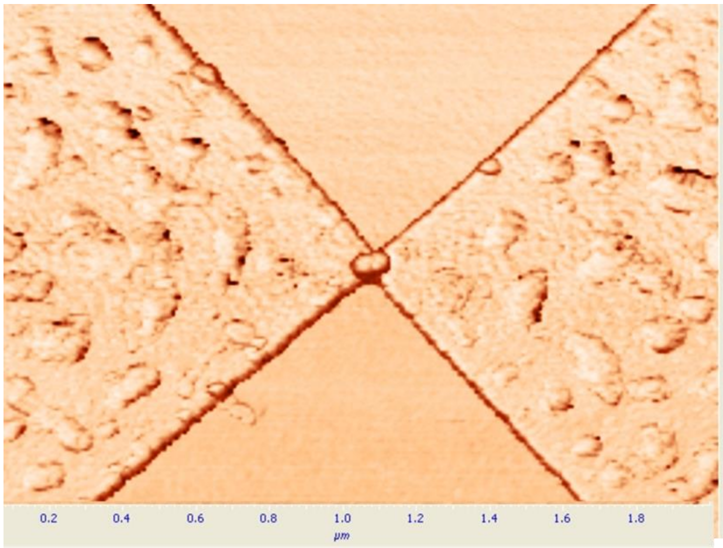


*Figure S5: AFM image of a trapped dimer*

## S2 Double dot simulation

The current through a double dot system can be written[5–7] as the difference between the forward and backward tunneling rates at each of the three tunnel barriers in the system:

$$I = |e| \sum_{(n_1,n_2)} P(n_1,n_2)[\gamma_i^+(n_1,n_2) - \gamma_i^-(n_1,n_2)]$$

Here, $e$ is the electron charge, $P(n_1,n_2)$ is the probability for finding the system with $n_1$ extra electrons in the first NP and $n_2$ extra electrons in the second NP, and $\gamma_i^\pm$ is the tunneling rate through the i'th barrier which is either in forward (+) or backward (-) direction.

The tunneling rate $\gamma_i$ is determined by the electrons' temperature T, the barrier conductivity $\mathrm{G}_i$, and the energy difference between the initial and final states of the system $\Delta\mathrm{E}_i$ (which is determined by the charging state $(n_1,n_2)$, the bias voltage $V_{SD}$, the back-gate voltage $V_G$ and the capacitances of the system) according to:

$$\gamma_i = \frac{G_i}{e^2}\frac{\Delta\mathrm{E}_i}{1 - Exp(-\Delta\mathrm{E}_i/k_B T)}$$

Using the Nelder-Mead simplex find method[8], we found the system's parameters (capacitances and three tunneling resistances) that best correspond to the measured results. In Figure S6 we present the measured conductance spectra and the corresponding fits for three devices: Devices A and B which are discussed in the main text, and Device C, which is characterized by a very slow switching RTS.

Device A:

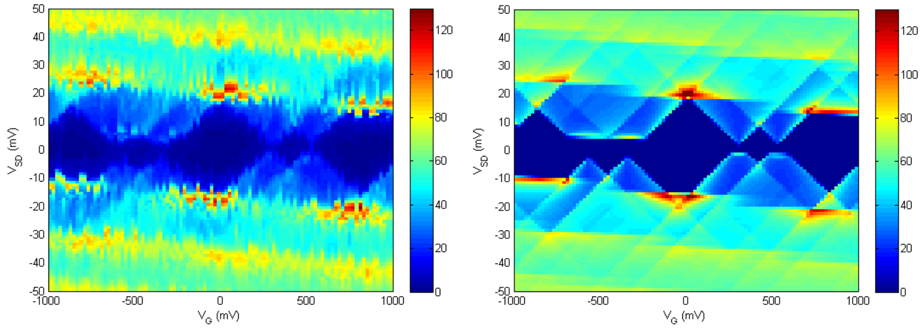


Device C:

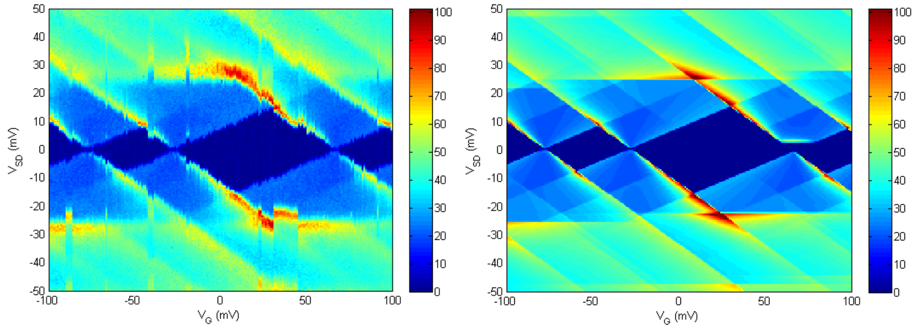


Device B:

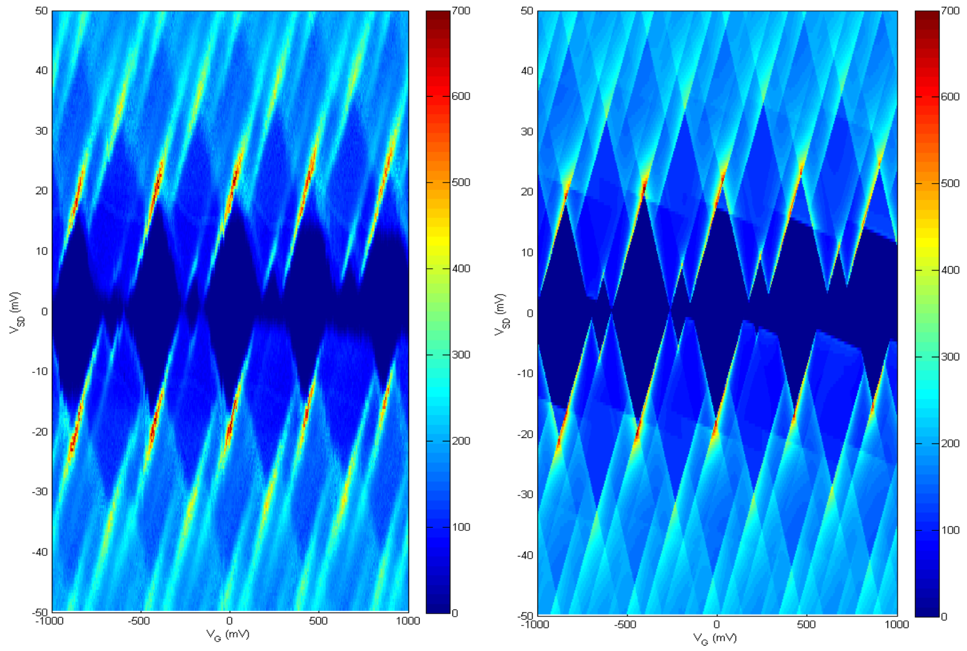


*Figure S6: Differential conductance (in nS) measurements (left) of three devices and their corresponding simulations (right). Devices A and B are discussed in the main text.*

## S2.1 Fit parameters

In Table S1 we show the fit parameters that were used to obtain the right panels in Fig. S6. $C_{i,j}$ and $R^{-1}_{i,j}$ are the capacitance (in aF) and conductance (in nS) between components i and j: L & R represent the left and right leads, 1 & 2 represent the two NPs and BG represents the back gate, respectively.

| Device | $C_{BG,1}$ | $C_{BG,2}$ | $C_{L,1}$ | $C_{1,2}$ | $C_{2,R}$ | $C_{L,2}$ | $C_{1,R}$ | $R^{-1}_{L,1}$ | $R^{-1}_{1,2}$ | $R^{-1}_{2,R}$ |
|---|---|---|---|---|---|---|---|---|---|---|
| A | 0.15 | 0.22 | 9.23 | 5.79 | 10.91 | 0.84 | 0.34 | 139 | 324 | 231 |
| B | 0.35 | 0.39 | 10.78 | 5.30 | 8.38 | 0.76 | 0.67 | 1092 | 333 | 1790 |
| C | 1.18 | 1.03 | 8.03 | 9.75 | 6.71 | 0.68 | 0.39 | 370 | 488 | 64 |

*Table S1: The fit parameters for Devices A, B, and C*

The main contributions to the capacitance come from the direct terms ($C_{L,1}$, $C_{2,R}$ and $C_{1,2}$), and are at most within a factor of 2 at the various devices. It is evident that the cross-capacitance terms ($C_{L,2}$, $C_{1,R}$) are an order of magnitude lower than the direct ones. The variation in conductance is larger, and may reach almost an order of magnitude.

The resulting charging energies[7] are given in Table S2.

| Device | $E_{C1}$ | $E_{C2}$ | $E_{CM}$ |
|---|---|---|---|
| A | 11.7 | 10.3 | 3.8 |
| B | 10.5 | 12.1 | 3.8 |
| C | 11.3 | 12.1 | 6.1 |

*Table S2: The individual and mutual charging energies of the NPs (*in meV)

## S2.2 Charging states

Using the same simulation with the best-fit parameters we extract the average charging state $(n_1, n_2)$ of the system at each value of $V_{SD}$ and $V_G$. It is instructive to look at the total charge, $\sum n = n_1 + n_2$, and the charge difference, $\delta n = n_1 - n_2$, see Fig. S7:

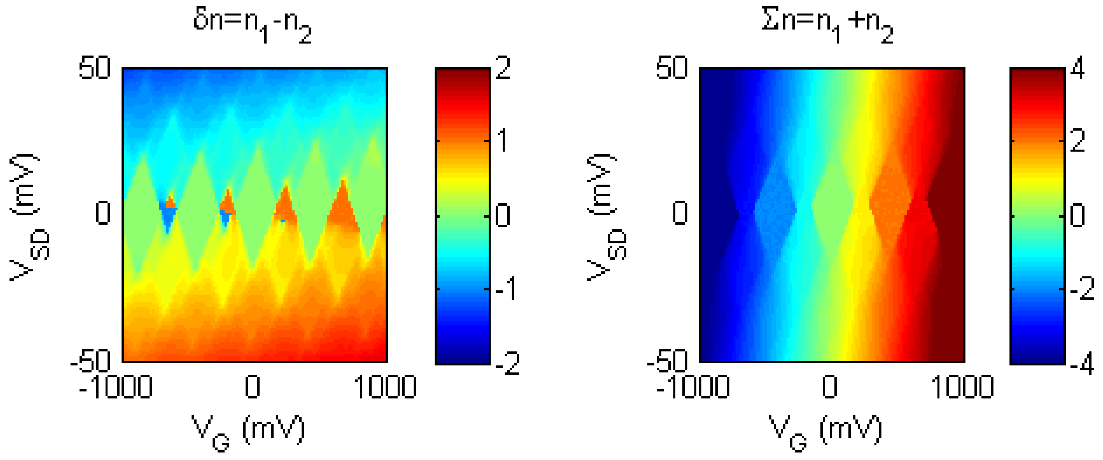


*Figure S7: The calculated total charge, $\sum n$, and charge difference, $\delta n$, for Device B in units of electron charge*

In Fig. S8 we show the relevant area, which is measured and shown in Fig. 2 of the main text.

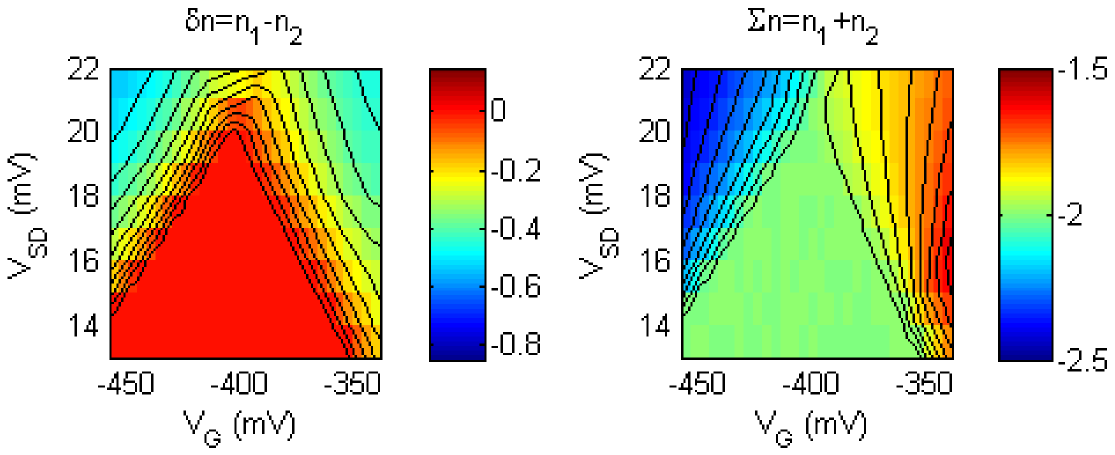


*Figure S8: A contour plot showing a zoom-in into the measured area of Device B*

We can now compare the calculated charging states with the clusters shown in the main text. We see that the two fast switching clusters (II and III) correspond to regions with the same charge difference, $\delta n$, and differ in their total charge, $\sum n$. On the other hand, the slow region near the blockade (region I) is characterized by $\delta n = 0$.

## S3 Trap dynamics

Consider a trap that can be either empty (0) or occupied (1). One can describe the rate equations for the occupation probability $P_{0,1}$ as:

$$\frac{dP_1}{dt} = \gamma_0 P_0(t) - \gamma_1 P_1(t)$$
$$\frac{dP_0}{dt} = -\gamma_0 P_0(t) + \gamma_1 P_1(t)$$
$$P_0(t) + P_1(t) = 1$$

where $\gamma_0 = \tau_0^{-1}$, $\gamma_1 = \tau_1^{-1}$ are the rates in which the trap is fed and emptied.

Solving these equations with an initial condition of $P_1(0) = 1$ provides the dynamics of the conditional probability:

$$P_{11} = Prob(state\ 1\ at\ time\ t \mid state\ 1\ at\ time\ 0) = \frac{\gamma_0 + e^{-t(\gamma_0+\gamma_1)}\gamma_1}{\gamma_0+\gamma_1}.$$

Similarly, the initial condition $P_0(0) = 1$ provides the conditional probability:

$$P_{00} = Prob(state\ 0\ at\ time\ t \mid state\ 0\ at\ time\ 0) = \frac{\gamma_1 + e^{-t(\gamma_0+\gamma_1)}\gamma_0}{\gamma_0+\gamma_1}.$$

### S3.1 Time auto-correlation function $g_2$

We define the normalized time auto-correlation function of a signal $I(t)$ as

$$g_2(\Delta t) = \frac{\langle \tilde{I}(t)\tilde{I}(t+\Delta t)\rangle}{\langle \tilde{I}^2(t)\rangle}$$

where $\tilde{I}(t) = I(t) - \langle I \rangle$ and $\langle \cdot \rangle$ represents time average.

Using the above probabilities and $I(t)$, which is due to the trap occupation state with the above dynamics, one can write:

$$\langle I(t)I(t+\Delta t)\rangle =$$
$$P_{0\infty}\left[a^2 P_{00}(\Delta t) + ab\left(1 - P_{00}(\Delta t)\right)\right] + P_{1\infty}\left[b^2 P_{11}(\Delta t) + ab\left(1 - P_{11}(\Delta t)\right)\right]$$

where $P_{0\infty} = \lim_{t\to\infty} P_{00}(t) = \frac{\gamma_1}{\gamma_0+\gamma_1}$, $P_{1\infty} = \lim_{t\to\infty} P_{11}(t) = \frac{\gamma_0}{\gamma_0+\gamma_1}$ and a,b are the values of the RTS corresponding to the trap occupation states 0,1, respectively.

It is now easy to calculate the normalized time auto-correlation function $g_2(\Delta t)$ for such signal, and get:

$$g_2(\Delta t) = \frac{\langle \tilde{I}(t)\tilde{I}(t+\Delta t)\rangle}{\langle \tilde{I}^2(t)\rangle} = exp[-\Gamma \cdot \Delta t]$$

where $\Gamma = \gamma_0 + \gamma_1$.

Hence, a trap that is fed in rate $\gamma_0 = \tau_0^{-1}$ and emptied in rate $\gamma_1 = \tau_1^{-1}$ is described by an exponential time auto-correlation function, $g_2$, with decay rate $\Gamma = \gamma_0 + \gamma_1$.

# S4 Measurements in the Coulomb Blockade

To test the limit for electron trapping we conducted measurements on Device B with $V_W$=0, deep in the blockade region and with no current flowing. These measurements were conducted using a similar sequence as in Fig. 4, using $V_G$=-400 mV and $V_M$=-16 mV. Figure S9 shows the results of 38 such measurements for various wait times $\Delta$t. For each value of $\Delta$t we have calculated the conditional probabilities, $P_{00}$ and $P_{11}$. These probabilities are shown as the blue points in Fig. S9. Remarkably, these probabilities remain the same over 4 orders of magnitude of $\Delta$t, and no decay is seen up to wait time of $\Delta$t=10 minutes.

The control measurement (green points) shows the conditional probabilities, when $V_W$= $V_M$=-16 mV. Here, as expected a clear exponential decay is seen (black solid curves are exponential fits to the points according to the equations for $P_{00}$ and $P_{11}$ in section S3).

We conclude that deep in the Coulomb blockade regime the decay rate $\Gamma$ is extremely long, and an electron can be trapped for a very long time when no current is flowing in the device.

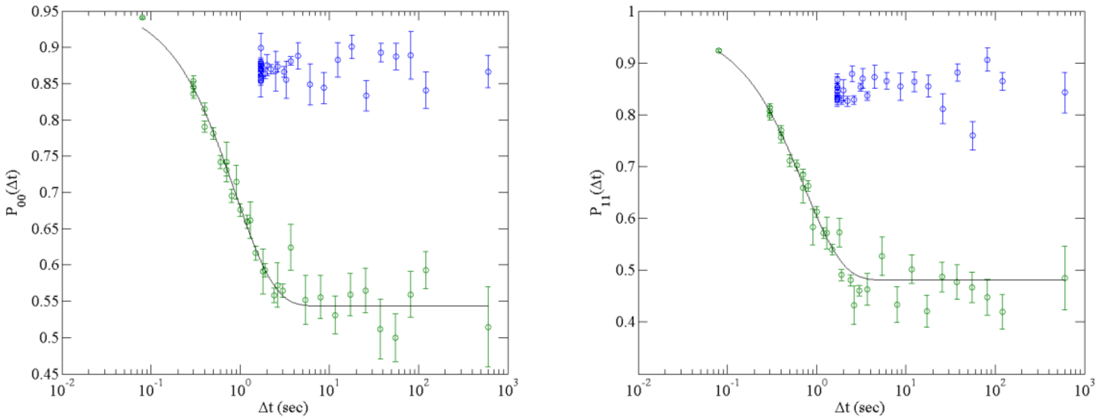


*Figure S9: The conditional probabilities, $P_{00}$ and $P_{11}$, as a function of the wait time $\Delta t$ at $V_{SD}$=$V_W$=0 (blue points) and $V_{SD}$=$V_W$=-16 mV (green points). The solid black curve is the expected exponential fit.*

## S5 Demonstration of Control

Here we demonstrate our ability to control the state of the trap, and actually 'write' its state and keep it for a long time. We keep the state of the trap in the 'off' (0) and 'on' (1) states, alternately, for 10 minutes. The red solid line indicates the desired state, while the blue dots are measurements of the system's state, shown on a normalized axis (measurement every 1 minute). All the measurements were done in the same $V_{SD}$, while between every 2 consecutive measurements we changed $V_{SD}$ to a different value, waited there for 1 minute, and thus fixed the state to either 'on' or 'off', according to the desired state (which we changed every 10 minutes). One can see the robustness and stability of the trap's state for over an hour.

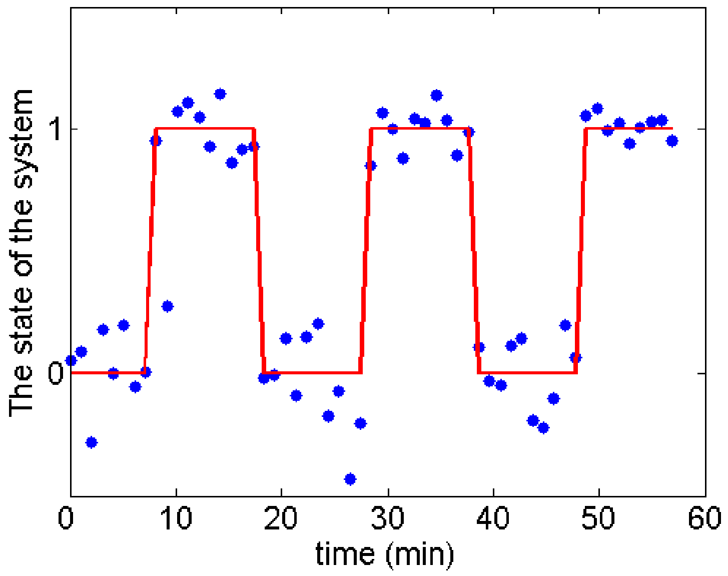


*Figure S10: Demonstration of the ability to 'read' and 'write' the trap state. We keep the state of the trap in the 'off' (0) and 'on' (1) states, alternately, for 10 minutes. The red solid line indicates the desired state, while the blue dots are measurements of the system's state (current), shown on a normalized axis.*

## S6 Numerical Calculations of the Trap Gating

We conducted a full numerical calculation of the induced gating of the two dots as a function of the trap location. The calculation was done using COMSOL Multiphysics 4.3. The geometry contained two metallic spheres with a diameter of 34 nm and a point charge with an electron charge that is located near them (a trapped electron). For each position of the trapped electron we calculated the voltage of each of the two spheres. We then got the change of voltage of the spheres as a function of the electron position, compared to the no electron case. Taking into account the fact that an electron can flow between a sphere and a lead when the electrochemical potential of the sphere is higher than that of the lead (as when current flows in the system), we got the total change of the electrochemical potential of each of the spheres compared to the unoccupied trap case, as a function of the location of the trapped electron. This change corresponds to a shift in the conductance spectrum, as mentioned in the main text.

Here we present this shift in a basis of common gating, $(\mu_1 + \mu_2)/2$, and differential gating, $(\mu_1 - \mu_2)/2$, where $\mu_1, \mu_2$ are the electrochemical potentials of the two spheres.

Note that a surface charge that is far away from the central region will not cause any significant effect, since it is equivalent to charging the dot by a full electron charge. On the other hand, a trapped charge in the center between the dots produces a differential gating with negligible common gating.

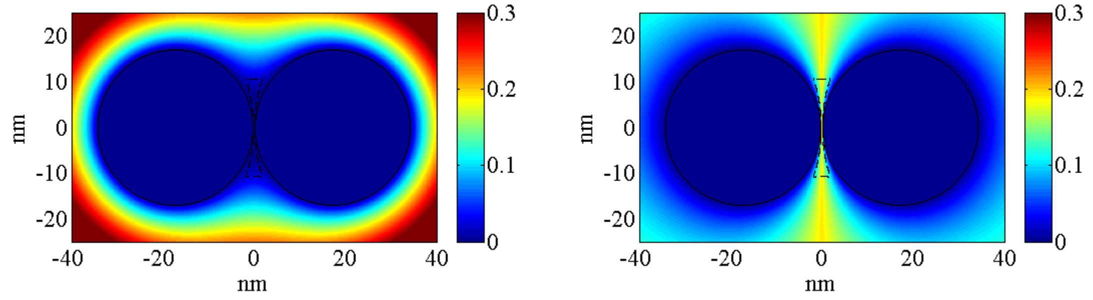


*Figure S11: Common gating (left) and differential gating (right) of the system, in units of the charging energy, $E_c$, as a function of the trap position. The marked area is the possible location of the trap in device A, which shows almost purely differential gating, as mentioned in the main text. It was defined as the area in which common gating<0.02$E_c$ and differential gating>0.1$E_c$. The sensitivity of the trap location to these threshold values was checked and found to be very low.*

## S7 References


(1) Slot, J. W.; Geuze, H. J. *Eur. J. Cell Biol.* **1985**, *38*, 87–93.

(2) Dadosh, T.; Gordin, Y.; Krahne, R.; Khivrich, I.; Mahalu, D.; Frydman, V.; Sperling, J.; Yacoby, A.; Bar-Joseph, I. *Nature* **2005**, *436*, 677–680.

(3) Guttman, A.; Mahalu, D.; Sperling, J.; Cohen-Hoshen, E.; Bar-Joseph, I. *Appl. Phys. Lett.* **2011**, *99*, 063113.

(4) Bezryadin, A.; Dekker, C.; Schmid, G. *Appl. Phys. Lett.* **1997**, *71*, 1273.

(5) Grabert, H.; Devoret, M. H. *Single Charge Tunneling: Coulomb Blockade Phenomena in Nanostructures:[Proceedings of the NATO Advanced Study Institute on Single Charge Tunneling, Held March 5-15, 1991, in Les Houches, France]*; Grabert, H.; Devoret, M. H., Eds.; Plenum Press: New York, 1992.

(6) Beenakker, C. W. J. *Phys. Rev. B* **1991**, *44*, 1646–1656.

(7) Van der Wiel, W.; De Franceschi, S.; Elzerman, J. M.; Fujisawa, T.; Tarucha, S.; Kouwenhoven, L. P. *Rev. Mod. Phys.* **2002**, *75*, 1–22.

(8) Nelder, J. A.; Mead, R. *Comput. J.* **1965**, *7*, 308–313.
